# Supplementary material for: Constraining the Absolute Orientation of Eta Carinae's Binary Orbit: A 3-D Dynamical Model for the Broad [Fe III] Emission
Source: arXiv:1111.2226 ancillary file (2011-11-09)
Supplement: Supplementary file 1 [file Supplementary_Materials_Appendices.pdf]

## APPENDIX A: MASKING PROCEDURE FOR THE *HST*/STIS OBSERVATIONS

Features in the observed spectro-images reveal at least three different formation environments for the forbidden lines that can be distinguished by their excitation and velocity profiles: the Weigelt blobs, the WWC structures, and the extended wind of $\eta_{\rm A}$. The Weigelt blobs are high-density, slow-moving ejecta from the 1890 eruption that contribute bright, narrow emission lines $\lesssim 50$ km s$^{-1}$ wide centered at $\sim -40$ km s$^{-1}$. In contrast, the broad high-ionization forbidden line emission originates in/near the spatially-extended WWC structures photoionized by $\eta_{\rm B}$. This material moves much faster, up to the terminal speed of $\eta_{\rm A}$'s wind. Broad, lower-ionization emission from lines of [Fe II] and Fe II forms in the extended wind of $\eta_{\rm A}$ and in portions of the WWC zones not photoionized by $\eta_{\rm B}$. The broad [Fe II] emission manifests itself as much more spatially-extended (up to $\pm 0.75''$) red- and blue-shifted double-arcs (see the far-right column of figures $11-13$ of G09).

Up to five narrow lines can contaminate the spectro-images of the broad [Fe III] $\lambda$4659 emission: Fe II $\lambda$4658; [Fe III] $\lambda$4659; N I $\lambda$4662; [Fe II] $\lambda$4666; and Fe II $\lambda$4668. The nearby [Fe II] $\lambda$4666 wind line also produces faint, broad contamination to the red in the [Fe III] $\lambda$4659 images. In order to facilitate the comparison of the synthetic spectro-images to the observations, we created a series of masked [Fe III] $\lambda$4659 spectro-images in which the contamination due to the nearby wind lines and Weigelt blobs has been concealed.

Laboratory wavelengths of lines identified in *HST*/STIS spectra of the Weigelt blobs were obtained from the atlas published by Zethson (2001) and Zethson et al. (2011). Relative strengths of these lines as noted in the individual spectro-images were confirmed by the Weigelt blob spectra published by Zethson (2001) and Zethson et al. (2011), recorded by *HST*/STIS in March 1998 (periastron), February 1999, and March 2000 (broad high state).

In each observed [Fe III] $\lambda$4659 spectro-image, we mask the narrow, $\sim 50$ km s$^{-1}$ wide [Fe III] $\lambda$4659 component that forms in the Weigelt blobs and is centered at $\sim -40$ km s$^{-1}$. We likewise mask the two narrow-line emission components centered at $\sim 520$ km s$^{-1}$ and $370$ km s$^{-1}$ that are due to Fe II $\lambda$4668 and [Fe II] $\lambda$4666, respectively. When present, the narrow Fe II $\lambda$4658 and N I $\lambda$4662 emission components centered at $\sim -110$ km s$^{-1}$ and $\sim +115$ km s$^{-1}$, respectively, are also masked. To determine the spatial and spectral ranges where faint, broad [Fe II] $\lambda$4666 wind emission contaminates the [Fe III] $\lambda$4659 image to the red, we use as a template the uncontaminated image of the bright [Fe II] $\lambda$4815 line, which we shift by $400$ km s$^{-1}$ to allow for direct comparison to the [Fe III] $\lambda$4659 image.

As an added check, we compare the observed spectro-images of [Fe III] $\lambda$4659 to those of [Fe III] $\lambda$4702 and [N II] $\lambda$5756, which form in nearly identical conditions since they have very similar critical densities and ionization potentials. The [Fe III] $\lambda$4702 and [N II] $\lambda$5756 images are useful for confirming the presence or absence of spatially-extended, red-shifted [Fe III] $\lambda$4659 emission. Unfortunately, images of [Fe III] $\lambda$4702 are contaminated to the red by the He I $\lambda$4714 wind line, which has a strong absorption component. However, the He I emission and absorption originate in the inner $0.1''$ core of $\eta$ Car. Absorption by He I $\lambda$4714 of the [Fe III] $\lambda$4702 emission is negligible and concentrated in the inner $0.1''$, leaving the spatially-extended emission relatively unaffected.

Since both [Fe III] $\lambda\lambda$4659 and 4702 are contaminated to the red by other lines, in most cases we also present spectro-images of [N II] $\lambda$5756. The [N II] $\lambda$5756 line is strong and located in a spectral region with very few other lines. Most importantly, there is no contamination to the red. With the exception of a narrow-line component centered at $\sim -450$ km s$^{-1}$ due to [Fe II] $\lambda$5748, and a narrow Weigelt-blob component at $\sim -40$ km s$^{-1}$, the [N II] $\lambda$5756 images are clean.

In the figures below, we present at each phase and slit PA the original, unmasked image of [Fe III] $\lambda$4659, the spectro-images of [Fe III] $\lambda$4702 and [Fe II] $\lambda$4815 used to define the mask, and the final masked image of [Fe III] $\lambda$4659 used in the paper for the comparison to the model spectro-image. When relevant and available, we also include the observed image of [N II] $\lambda$5756. All spectro-images have been processed identically with a spatial row-by-row continuum subtraction using a portion of the spectrum with no bright narrow- or broad-line contamination. Because the row-by-row continuum subtraction across the stellar position is poor due to insufficient correction in the data reduction for small tilts of the spectrum on the CCD (G09), we have left the inner $0.1''$ core of the observed spectro-images unmasked.

### A1 Emission Arcs at Slit PA = $+38^{\circ}$, $\phi = 0.976$

Figure A1 displays observed spectro-images of [Fe III] $\lambda$4659, [Fe II] $\lambda$4815, [Fe III] $\lambda$4702, and [N II] $\lambda$5756, all recorded at slit PA = +38° and phase $\phi = 0.976$. The [Fe III] $\lambda$4659 shows spatially-extended (up to $\sim 0.35''$) emission in the form of a pair of very distinct arcs that are entirely blue-shifted, up to $\sim -500$ km s$^{-1}$. While no other highly excited forbidden line shows a spatially-extended ($> 0.1''$) red component at this orbital phase and slit PA, we are unable to show a completely isolated line of [Fe III]. Several weaker [Fe III] lines nearby in the spectrum, while blended, show no evidence of a spatially-extended red component. The image of [Fe III] $\lambda$4702 demonstrates this. The strong absorption component of He I $\lambda$4714 is clearly visible in the central $0.1''$ core stretching in velocity from $\sim 100$ km s$^{-1}$ to $400$ km s$^{-1}$. Some faint He I $\lambda$4714 emission is also seen as scattered light extending $\sim 0.3''$ to the SW at velocities between $\sim 450$ km s$^{-1}$ and $600$ km s$^{-1}$. However, there is no spatially-extended, red-shifted $\lambda$4702 emission. The blue-shifted emission is very similar in structure to that in the [Fe III] $\lambda$4659 image.

The [N II] $\lambda$5756 image, not contaminated to the red, also shows no spatially-extended, red-shifted emission. The absence of extended, red-shifted [N II] strongly supports the absence of extended, red-shifted [Fe III]. The structure of the [N II] blue-shifted emission is nearly identical to that in the two [Fe III] images.

Faint emission to the red between $\sim 0$ and 600 km s$^{-1}$ in the [Fe III] $\lambda$4659 image is entirely due to contamination by [Fe II] $\lambda$4666, as illustrated by the velocity-shifted image of [Fe II] $\lambda$4815. The shape and structure of the faint red emission in the [Fe III] $\lambda$4659 image is identical to that of the brighter [Fe II] $\lambda$4815 line. Thus, based on the observations, we define the mask to extend from $\pm 0.1''$ to $\pm 1.0''$, and from $\sim -70$ km s$^{-1}$ to $+600$ km s$^{-1}$.

### A2 Variations with Phase for Constant Slit PA = $-28^{\circ}$

Figures A2 through A7 display observed spectro-images of [Fe III] $\lambda$4659, [Fe II] $\lambda$4815, and [Fe III] $\lambda$4702 as a function of orbital phase for slit PA = $-28^{\circ}$. At this PA, the faint contamination to the red in the [Fe III] $\lambda$4659 images that is due to [Fe II] $\lambda$4666 is much weaker and concentrated to the SE. The main sources of contamination are the narrow-line emission components that originate in the Weigelt blobs. Note the two narrow components from Fe II $\lambda$4658 and N I $\lambda$4662 centered at $\sim -110$ km s$^{-1}$ and

$\sim +115\ \mathrm{km\,s^{-1}}$, respectively, that are especially prominent in images of $\lambda$4659 taken during periastron (Figures A2 and A6). These are not present in the observations of Figure A1, or the spectro-images of [Fe III] $\lambda$4702. Moreover, because they remain bright during periastron (Zethson 2001; Zethson et al. 2011), they cannot be a result of high-ionization forbidden line emission. We thus mask both of these features. The [Fe III] $\lambda$4702 images in Figures A2 and A6 help to further demonstrate the disappearance of the spatially-extended [Fe III] emission during periastron, without the narrow-line contamination.

Unfortunately, the narrow N I $\lambda$4662 emission component complicates spectro-images of [Fe III] $\lambda$4659 at phases far from periastron (Figures A3 - A5 and A7), which show spatially-extended, red-shifted emission stretching to the NW at velocities between $\sim 0$ and up to $250\ \mathrm{km\ s^{-1}}$. There is little to no [Fe II] contamination in this direction at these velocities, as shown in the [Fe II] $\lambda$4815 images. Spectro-images of [Fe III] $\lambda$4702 (Figures A3 - A5 and A7) and [N II] $\lambda$5756 (Figures A3, A5, and A7) confirm that the spatially-extended, red-shifted [Fe III] $\lambda$4659 emission to the NW is real. We thus use the [Fe III] $\lambda$4702 and [N II] $\lambda$5756 images to help determine the spatial and spectral extents of the masks on the red side of the [Fe III] $\lambda$4659 line so as to ensure that we do not accidentally mask any broad, spatially-extended, red-shifted [Fe III] $\lambda$4659 emission. However, it is important to keep in mind that extended [Fe III] $\lambda$4659 emission at velocities between $\sim 90\ \mathrm{km\,s^{-1}}$ and $140\ \mathrm{km\ s^{-1}}$ may be contaminated by some faint, narrow N I $\lambda$4662 emission. This mostly leads to a baseline offset in the total flux and does not affect our overall conclusions.

### A3 Doppler Shift Correlations with Phase and Slit PA

Figures A8 through A17 present spectro-images of [Fe III] $\lambda$4659, [Fe II] $\lambda$4815, and [Fe III] $\lambda$4702 as a function of orbital phase and slit PA. Additional spectro-images of [N II] $\lambda$5756 are included for phases away from periastron. As with Figures A1 through A7, in each observed $\lambda$4659 spectro-image, we mask the narrow-line emission from the Weigelt blobs that is due to [Fe III] $\lambda$4659 (centered at $-40\ \mathrm{km\ s^{-1}}$), Fe II $\lambda$4668 (at $+520\ \mathrm{km\ s^{-1}}$), [Fe II] $\lambda$4666 (at $+370\ \mathrm{km\ s^{-1}}$), and, when present, Fe II $\lambda$4658 (at $-110\ \mathrm{km\ s^{-1}}$) and N I $\lambda$4662 (at $+115\ \mathrm{km\ s^{-1}}$). Faint, broad emission to the red due to the [Fe II] $\lambda$4666 wind line is also masked based on the images of [Fe II] $\lambda$4815.

Observation taken at $\phi = 0.601$, PA = +22° (Figure A8); $\phi = 0.984$, PA = +62° (Figure A13); and $\phi = 0.995$, PA = +70° (Figure A14) show two additional narrow emission components centered at velocities of $\sim -80\ \mathrm{km\,s^{-1}}$ and $-140\ \mathrm{km\,s^{-1}}$. Both of these narrow components are present in the corresponding [Fe III] $\lambda$4702 and [N II] $\lambda$5756 spectro-images, meaning that they represent real, narrow high-ionization forbidden line emission, as opposed to contamination from nearby narrow, low-ionization lines. The exact origin of these two features is uncertain, but given their slow speed (relative to $\eta_{\mathrm{A}}$'s wind) and narrow velocity width, they very likely represent dense, slow-moving ejecta between or around the Weigelt blobs that was also ejected sometime around 1890. As such, we mask out these narrow features. The $\phi = 0.820$, $\mathrm{PA} = +69°$ observation (Figure A10) also exhibits the $-80\ \mathrm{km\ s^{-1}}$ narrow component, but not the $-140\ \mathrm{km\,s^{-1}}$ component.

Finally, we note that the spatially-extended, red-shifted emission to the NW in spectro-images of [Fe III] $\lambda$4659 at $\phi = 0.738$, PA = -82° (Figure A9) and $\phi = 0.930$, PA = -57° (Figure A11) is real and extends in velocity from $\sim 0$ to $+250\ \mathrm{km\,s^{-1}}$, as demonstrated in the [Fe III] $\lambda$4702 and [N II] $\lambda$5756 images.

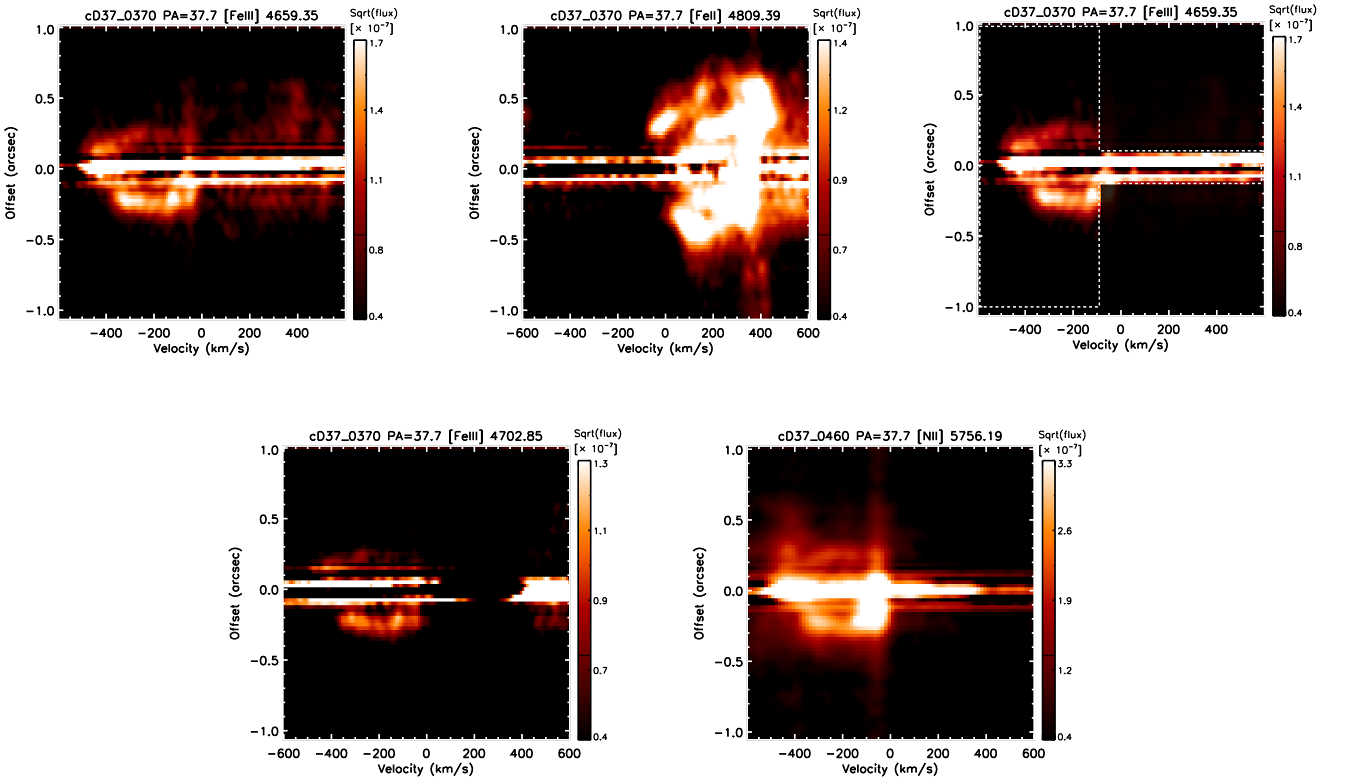


**Figure A1.** Spectro-images recorded 2003 May 5 ($\phi = 0.976$) at STIS slit PA $= +38°$. In all spectro-images of this figure and those that follow, the color scale is proportional to the square root of the intensity and the velocity scale is $\pm 600$ km s$^{-1}$. *Top Row, Left Panel*: Original, continuum-subtracted spectro-image of [Fe III] $\lambda$4659. Emission appears as a pair of entirely blue-shifted arcs. Weak emission to the red is entirely due to contamination by [Fe II] $\lambda$4666. Weak, narrow emission centered at $\sim -40$ km s$^{-1}$ comes from the nearby Weigelt blobs. *Top Row, Middle Panel*: Spectro-image of [Fe II] $\lambda$4815, shifted by 400 km s$^{-1}$, used to determine the spatial and spectral extent of the [Fe II] $\lambda$4666 contamination in the [Fe III] $\lambda$4659 image. *Top Row, Right Panel*: Masked spectro-image of [Fe III] $\lambda$4659. *Bottom Row*: Spectro-images of [Fe III] $\lambda$4702 (left panel) and [N II] $\lambda$5756 (right panel), included in order to demonstrate that the high-ionization forbidden lines observed at this phase and STIS PA show no evidence of spatially-extended, red-shifted emission.

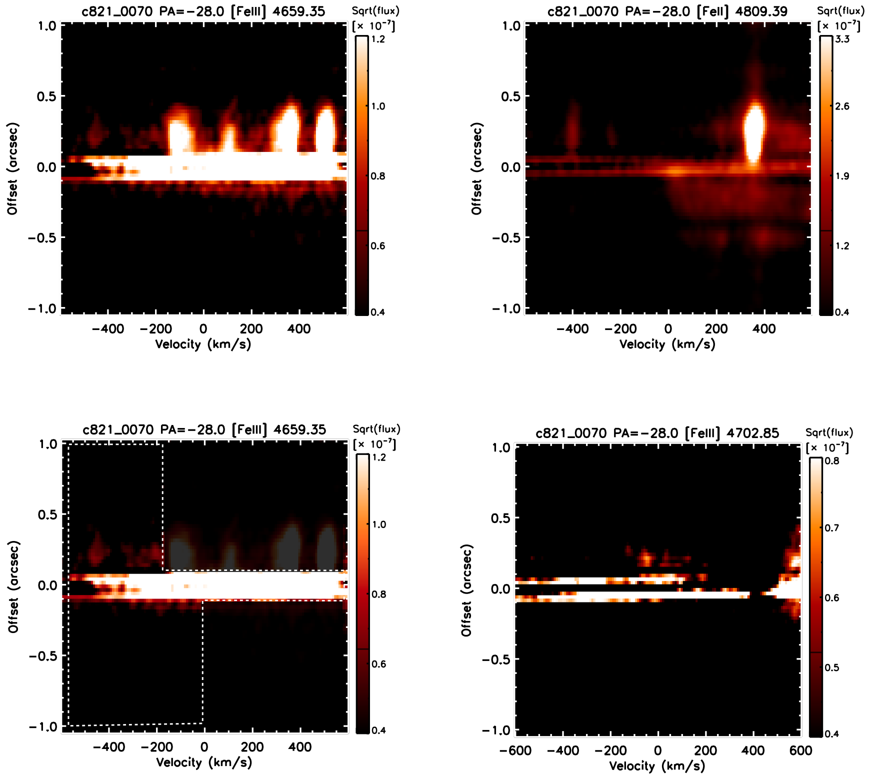


**Figure A2.** Spectro-images recorded 1998 March 19 ($\phi = 0.045$) at STIS slit PA $= -28°$. *Top Row*: Original, continuum-subtracted spectro-image of [Fe III] $\lambda$4659 (left panel) and spectro-image of [Fe II] $\lambda$4815, shifted by $400$ km s$^{-1}$ (right panel). *Bottom Row*: Masked spectro-image of [Fe III] $\lambda$4659 (left panel) and original spectro-image of [Fe III] $\lambda$4702 (right panel).

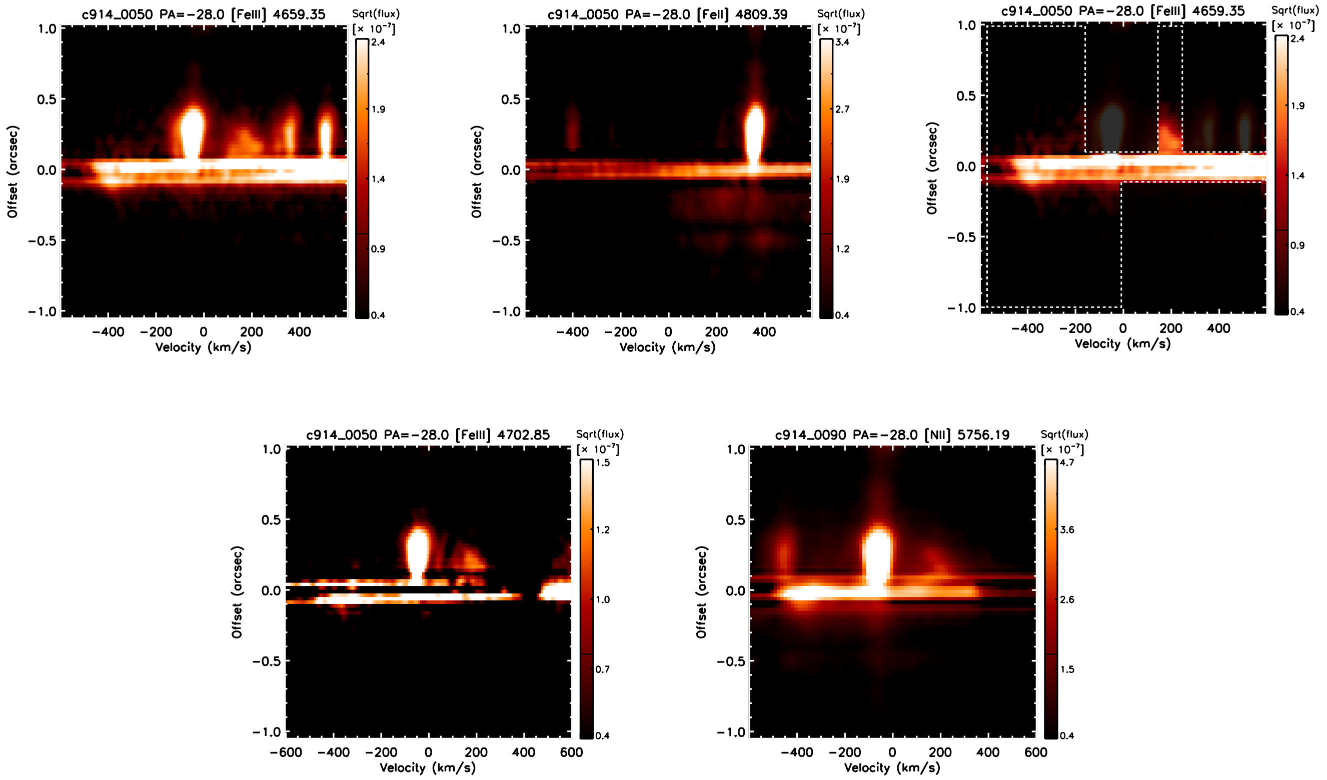


**Figure A3.** Spectro-images recorded 1999 February 21 ($\phi = 0.213$) at STIS slit PA $= -28°$. *Top Row, Left Panel*: Original, continuum-subtracted spectro-image of [Fe III] $\lambda$4659. *Top Row, Middle Panel*: Spectro-image of [Fe II] $\lambda$4815, shifted by $400$ km s$^{-1}$. *Top Row, Right Panel*: Masked spectro-image of [Fe III] $\lambda$4659. *Bottom Row*: Spectro-images of [Fe III] $\lambda$4702 (left panel) and [N II] $\lambda$5756 (right panel).

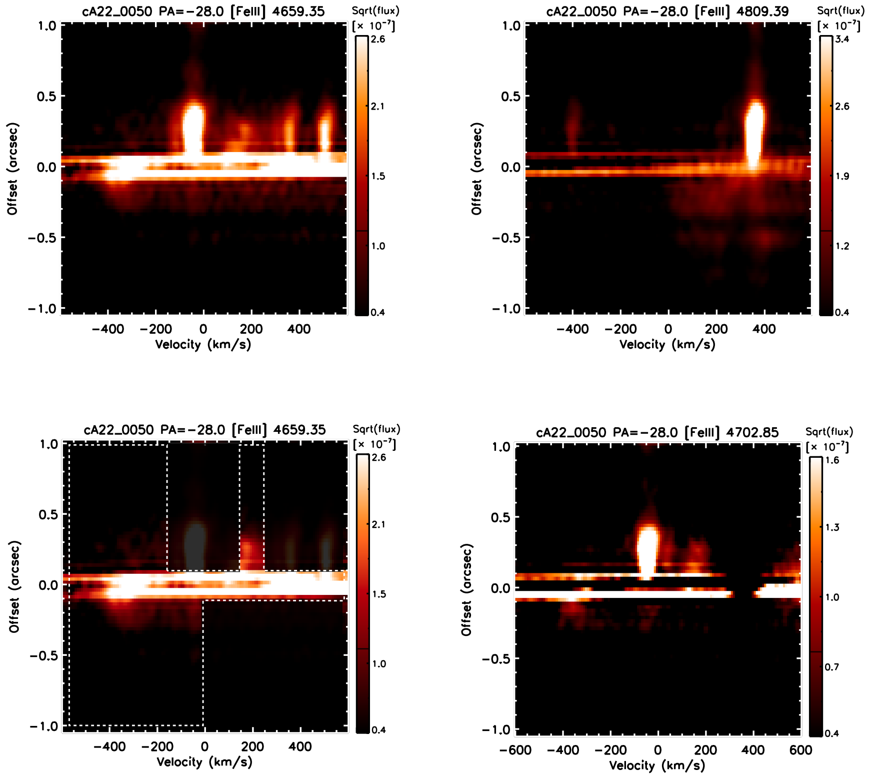


**Figure A4.** Same as Figure A2, but for spectro-images recorded 2000 March 20 ($\phi = 0.407$) at STIS slit PA $= -28°$.

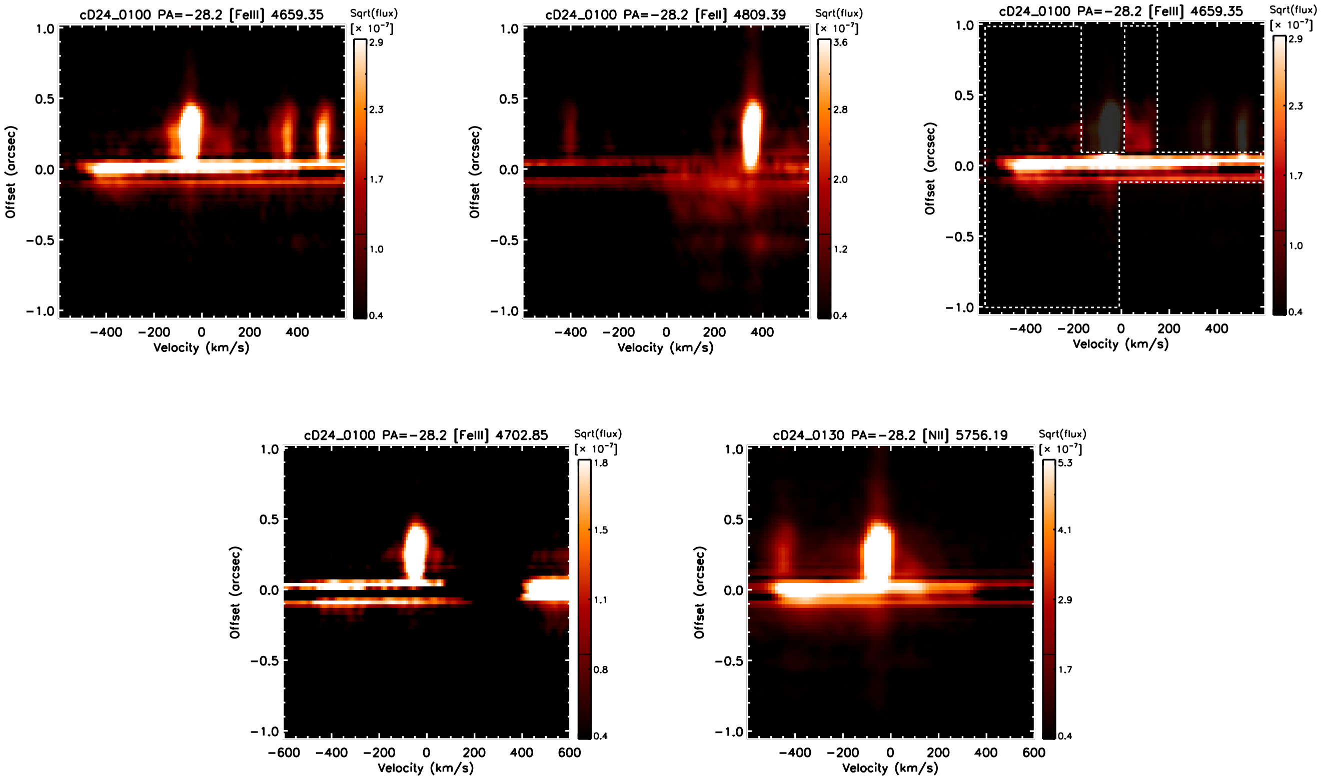


**Figure A5.** Same as Figure A3, but for spectro-images recorded 2003 March 29 ($\phi = 0.952$) at STIS slit PA $= -28°$.

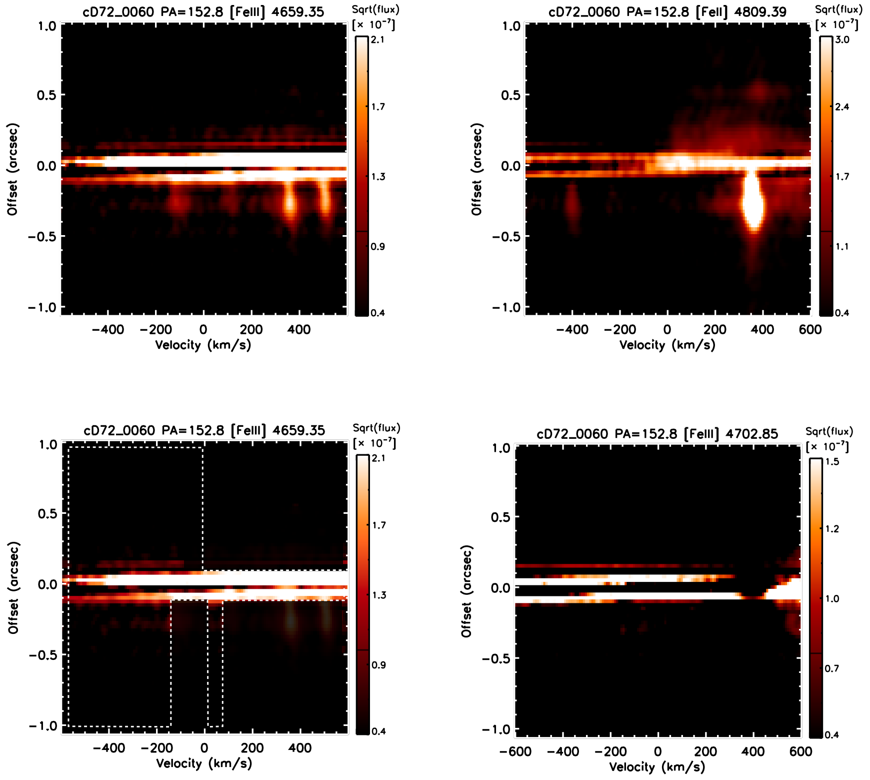


**Figure A6.** Same as Figures A2 and A4, but for spectro-images recorded 2003 September 22 ($\phi = 1.040$) at STIS slit PA $= +153°$.

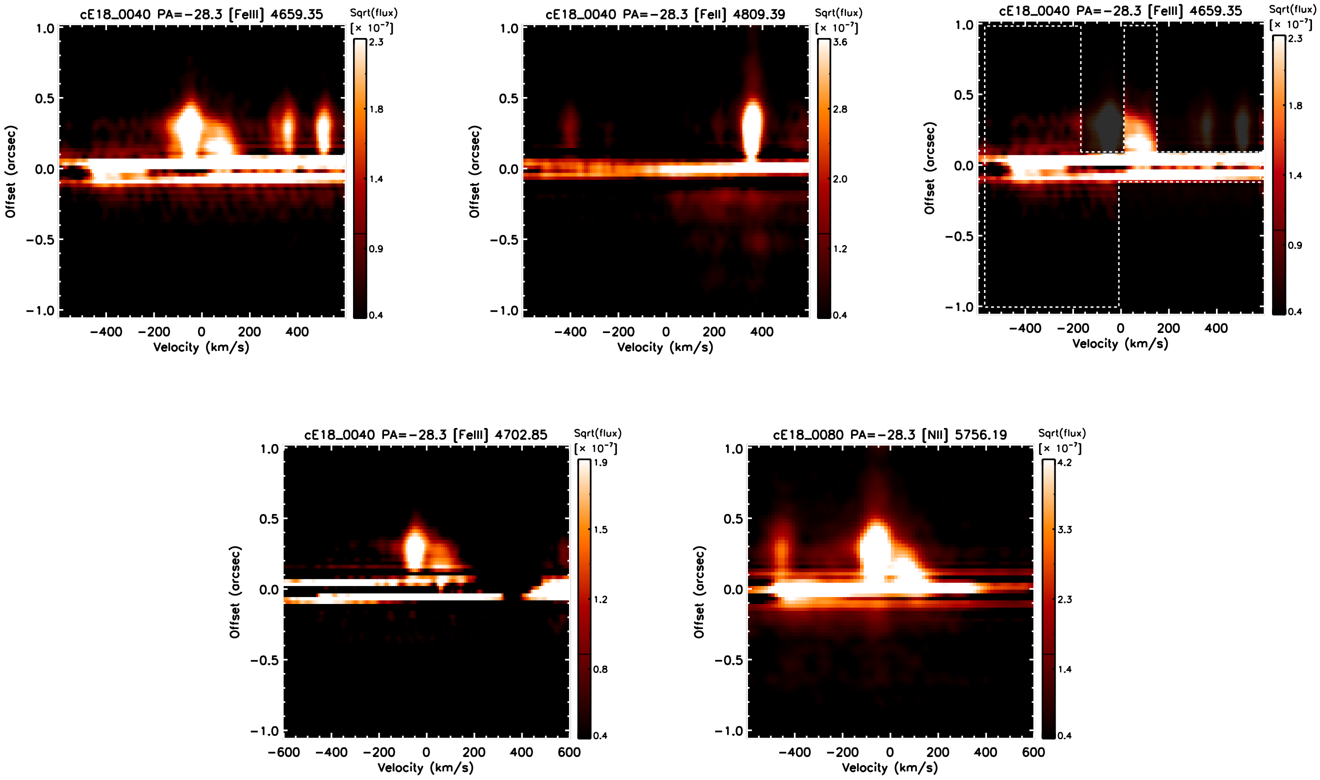


**Figure A7.** Same as Figures A3 and A5, but for spectro-images recorded 2004 March 6 ($\phi = 1.122$) at STIS slit PA $= -28°$.

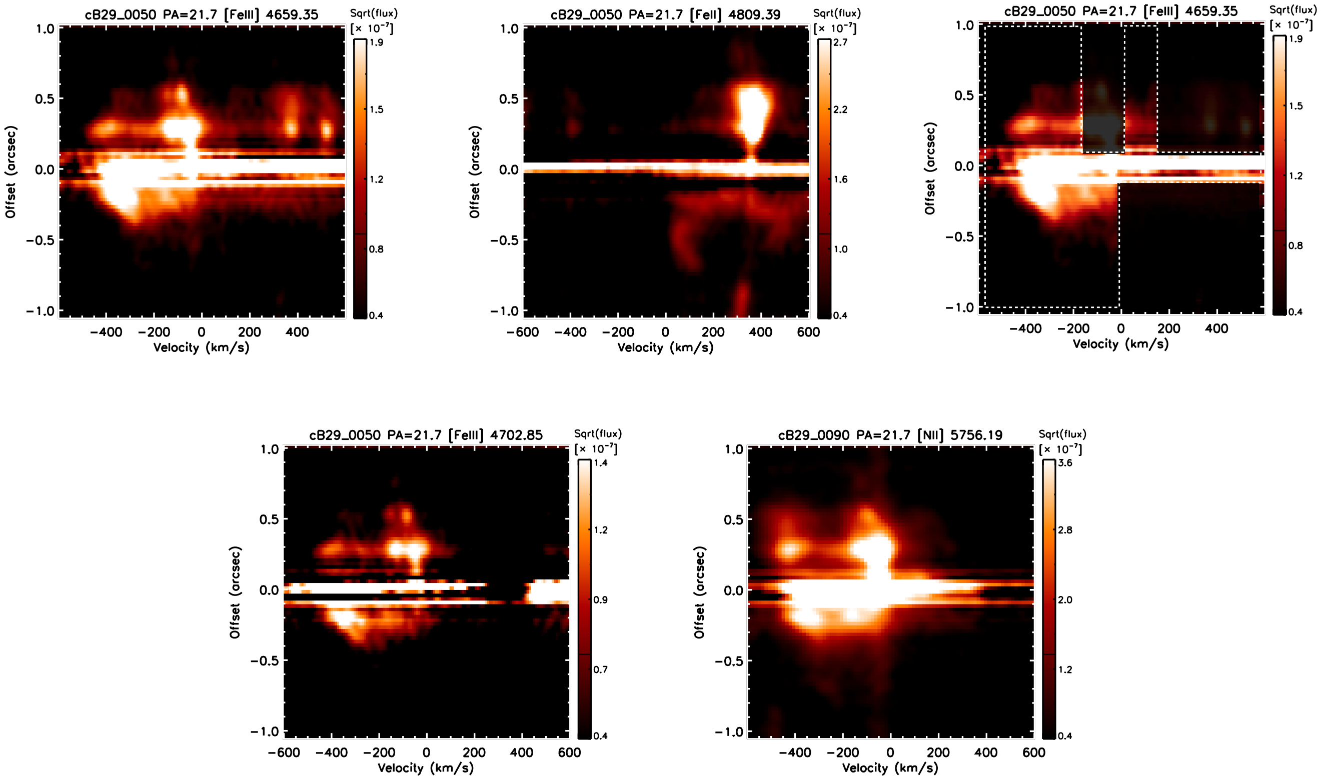


**Figure A8.** Spectro-images recorded 2001 April 21 ($\phi = 0.601$) at STIS slit PA $= +22°$. *Top Row, Left Panel*: Original, continuum-subtracted spectro-image of [Fe III] $\lambda$4659. *Top Row, Middle Panel*: Spectro-image of [Fe II] $\lambda$4815, shifted by $400$ km s$^{-1}$. *Top Row, Right Panel*: Masked spectro-image of [Fe III] $\lambda$4659. *Bottom Row*: Spectro-images of [Fe III] $\lambda$4702 (left panel) and [N II] $\lambda$5756 (right panel).

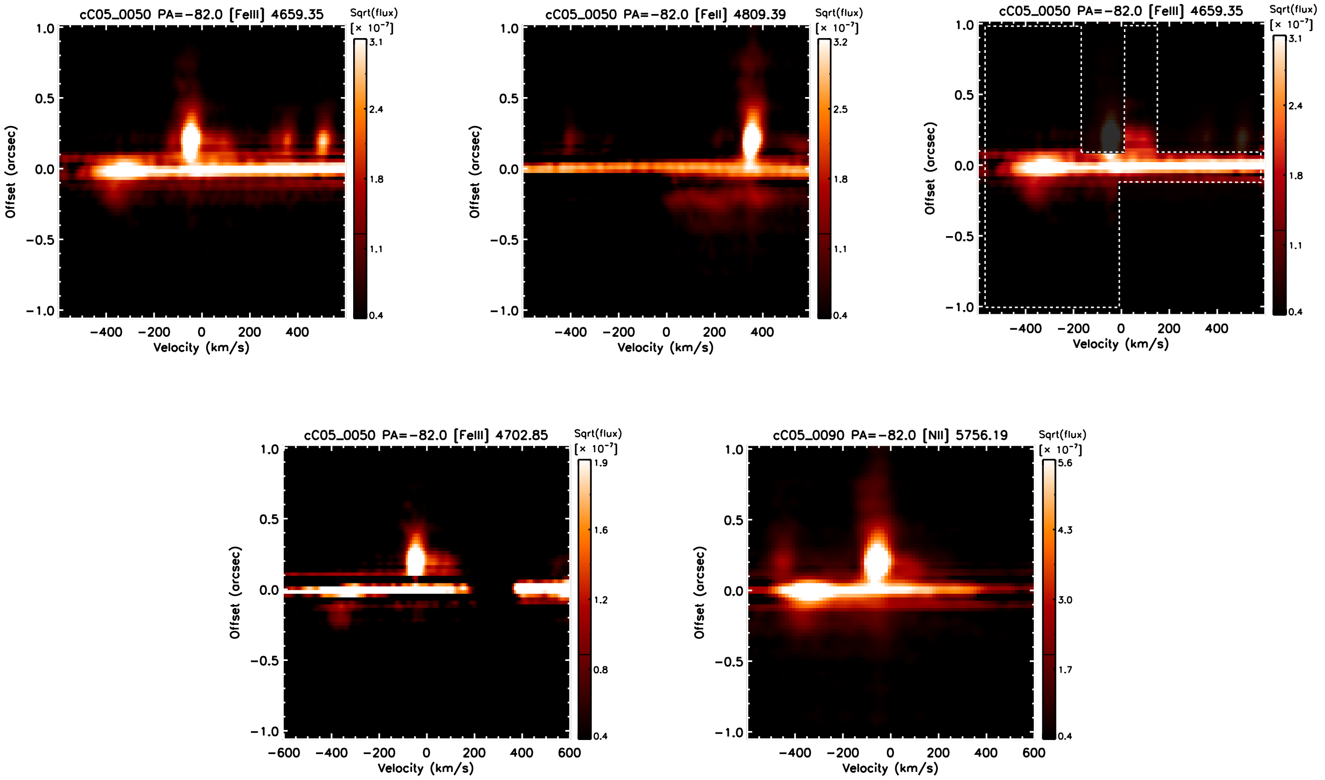


**Figure A9.** Same as Figure A8, but for spectro-images recorded 2002 January 19 ($\phi = 0.738$) at STIS slit PA $= -82°$.

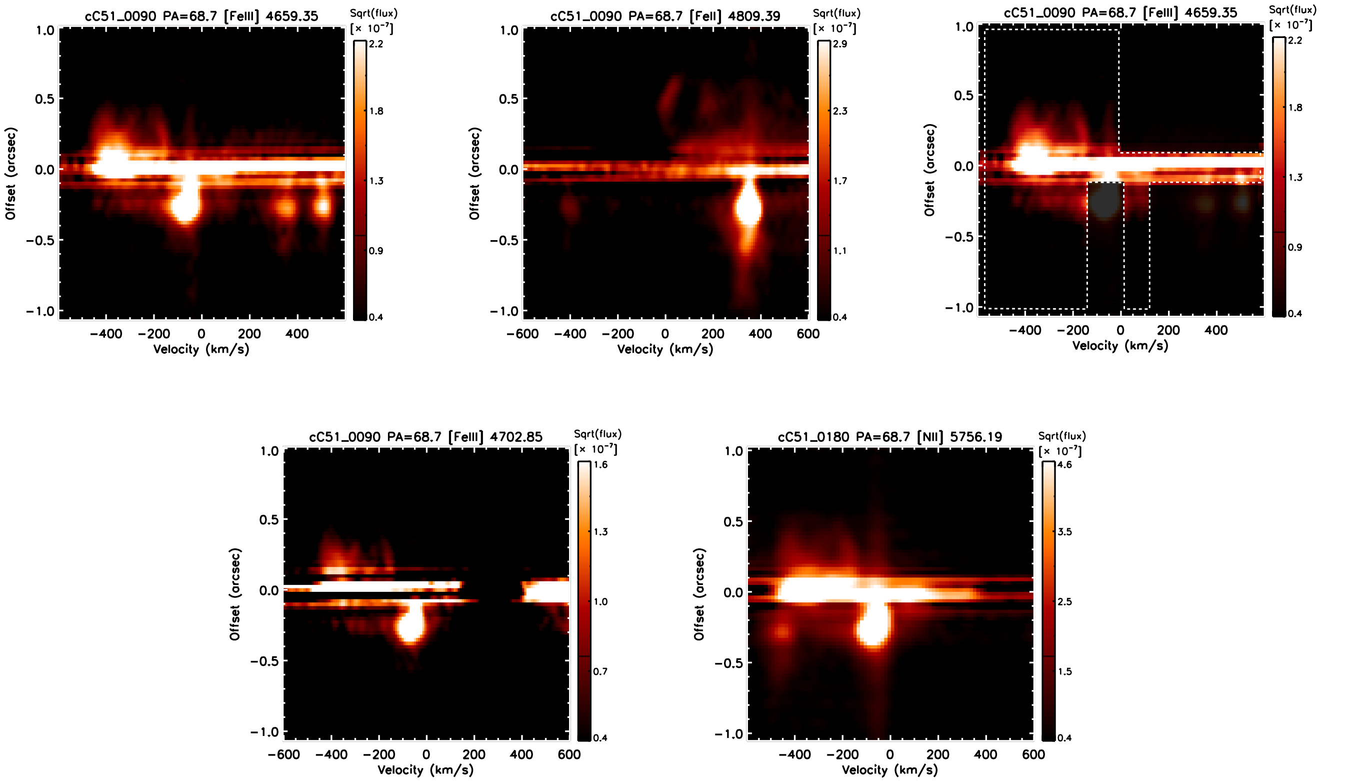


**Figure A10.** Same as Figures A8 and A9, but for spectro-images recorded 2002 July 4 ($\phi = 0.820$) at STIS slit PA $= +69°$.

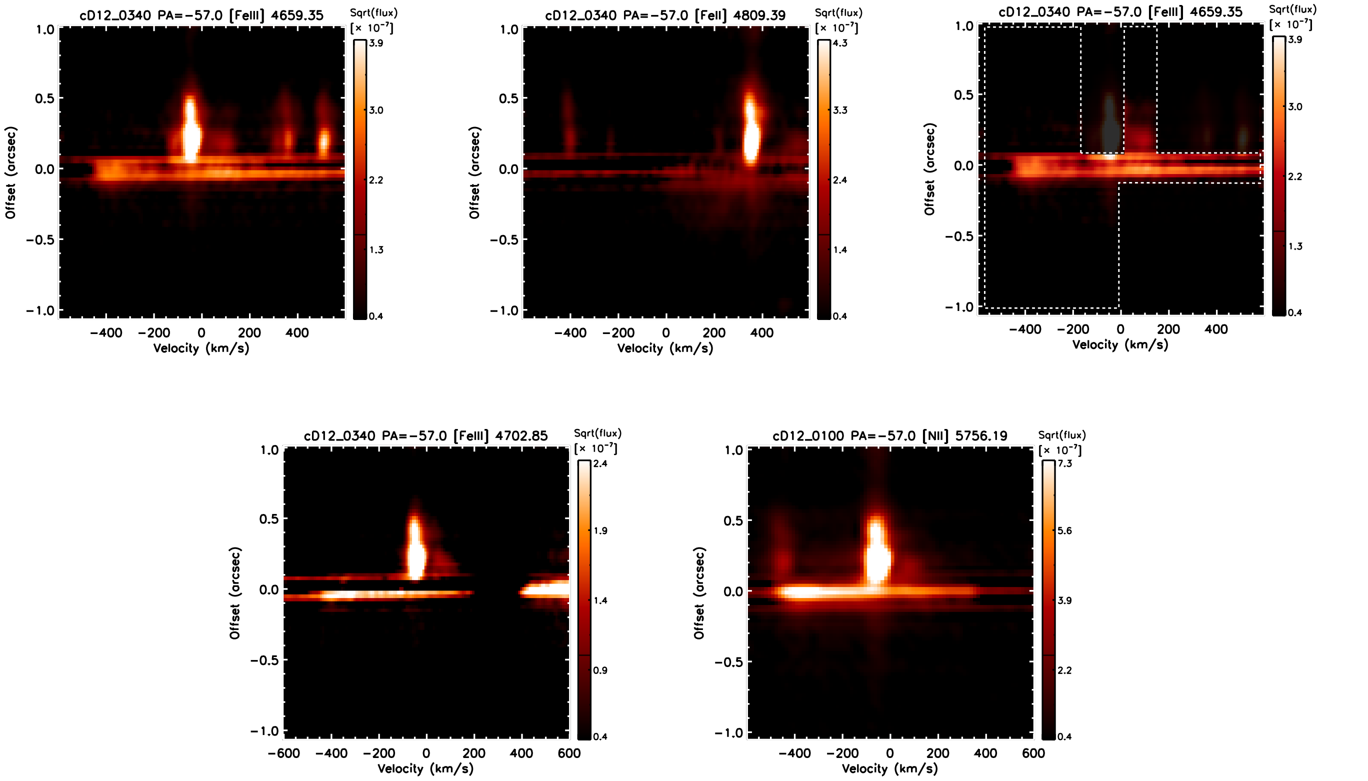


**Figure A11.** Same as Figures A8 through A10, but for spectro-images recorded 2003 February 12 ($\phi = 0.930$) at STIS slit PA $= -57°$.

© 0000 RAS, MNRAS **000**, 000–000

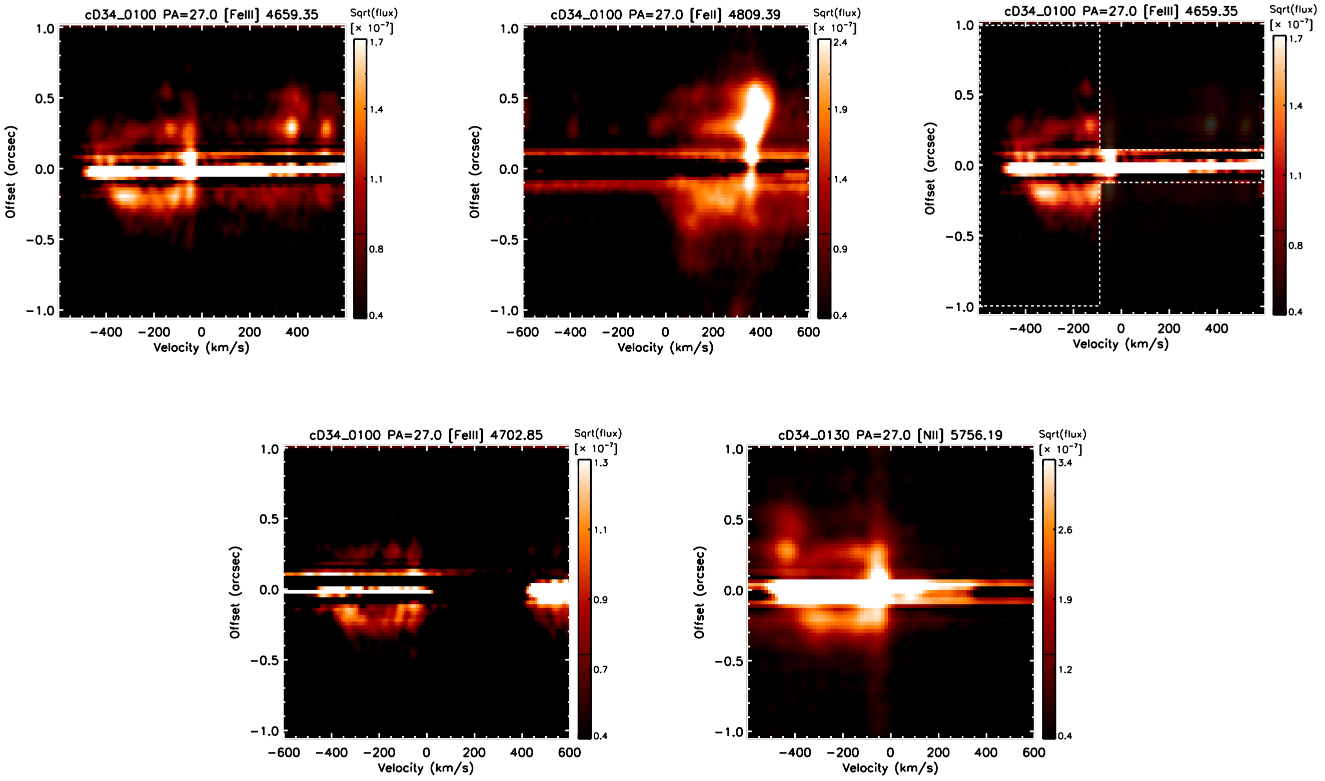


**Figure A12.** Same as Figures A8 through A11, but for spectro-images recorded 2003 May 5 ($\phi = 0.970$) at STIS slit PA $= +27°$.

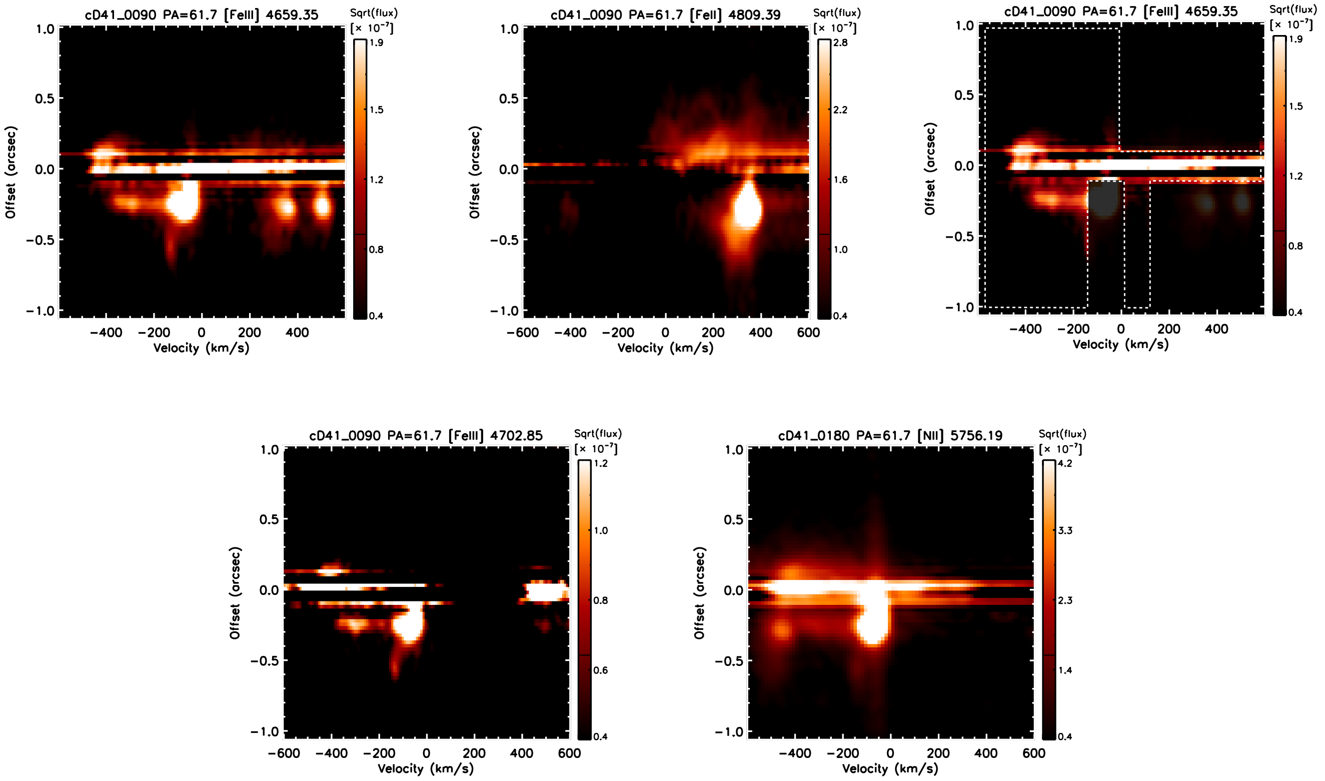


**Figure A13.** Same as Figures A8 through A12, but for spectro-images recorded 2003 June 1 ($\phi = 0.984$) at STIS slit PA $= +62°$.

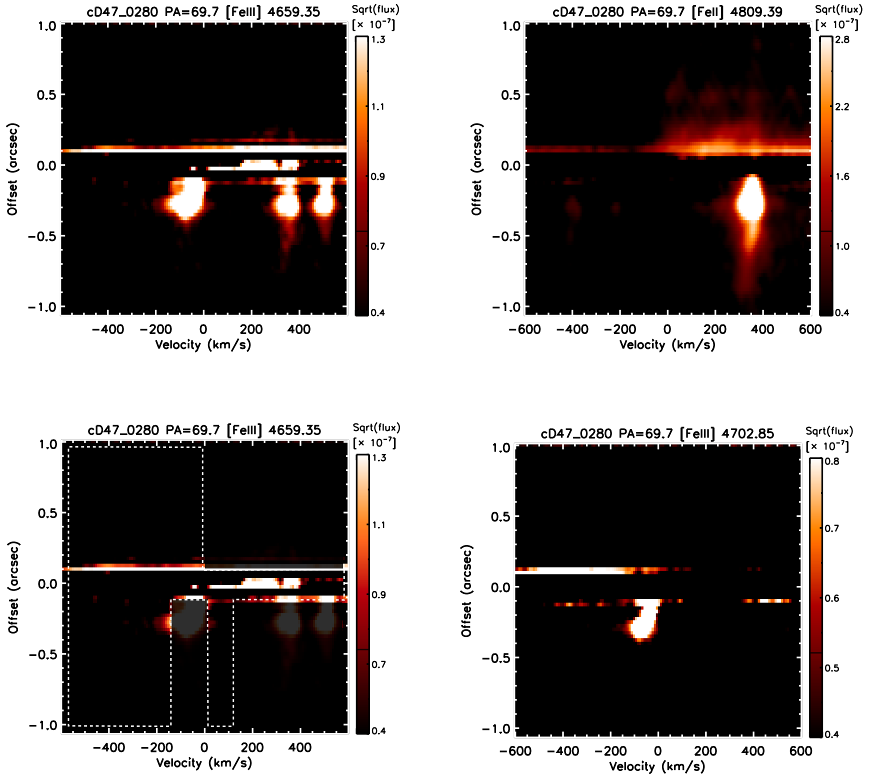


**Figure A14.** Spectro-images recorded 2003 June 22 ($\phi = 0.995$) at STIS slit PA $= +70°$. *Top Row*: Original, continuum-subtracted spectro-image of [Fe III] $\lambda$4659 (left panel) and spectro-image of [Fe II] $\lambda$4815, shifted by $400\ \mathrm{km\ s^{-1}}$ (right panel). *Bottom Row*: Masked spectro-image of [Fe III] $\lambda$4659 (left panel) and original spectro-image of [Fe III] $\lambda$4702 (right panel).

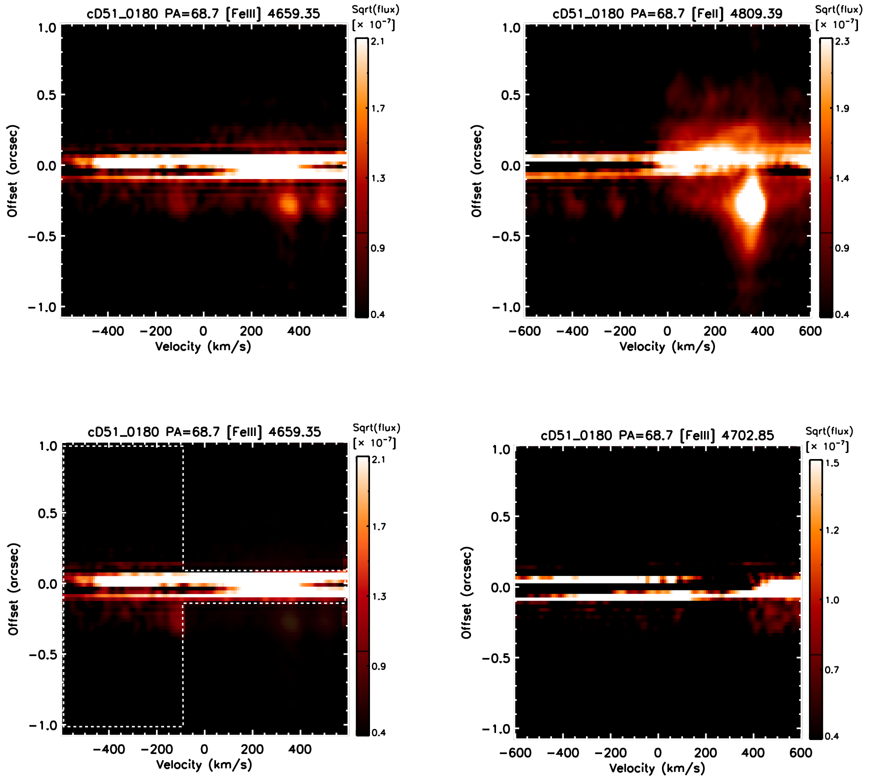


**Figure A15.** Same as Figure A14, but for spectro-images recorded 2003 July 5 ($\phi = 1.001$) at STIS slit PA $= +69°$.

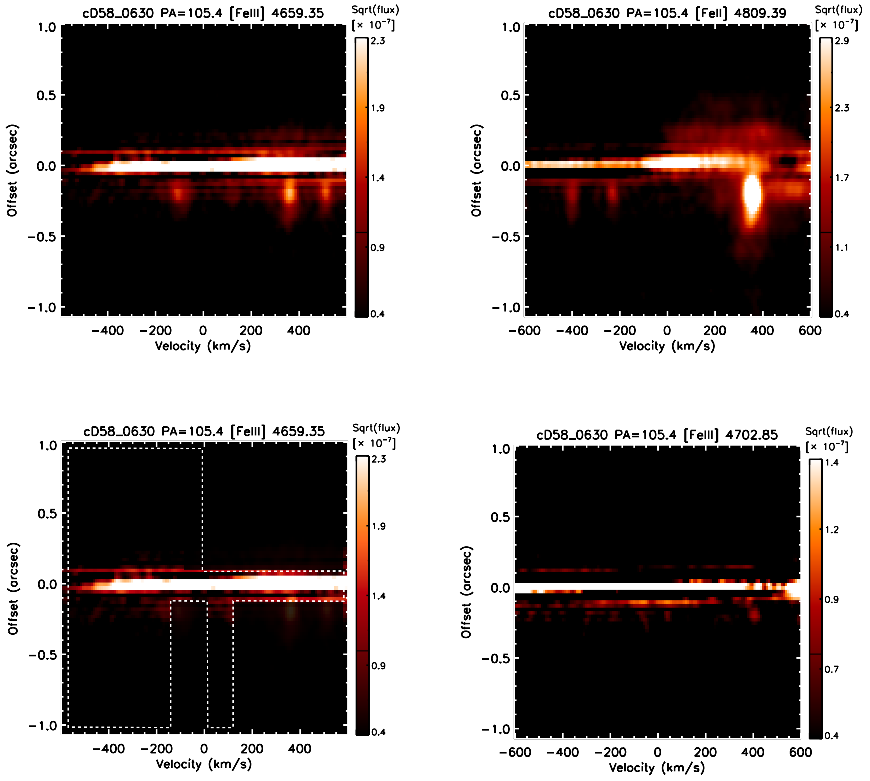


**Figure A16.** Same as Figures A14 and A15, but for spectro-images recorded 2003 July 29 ($\phi = 1.013$) at STIS slit PA $= +105°$.

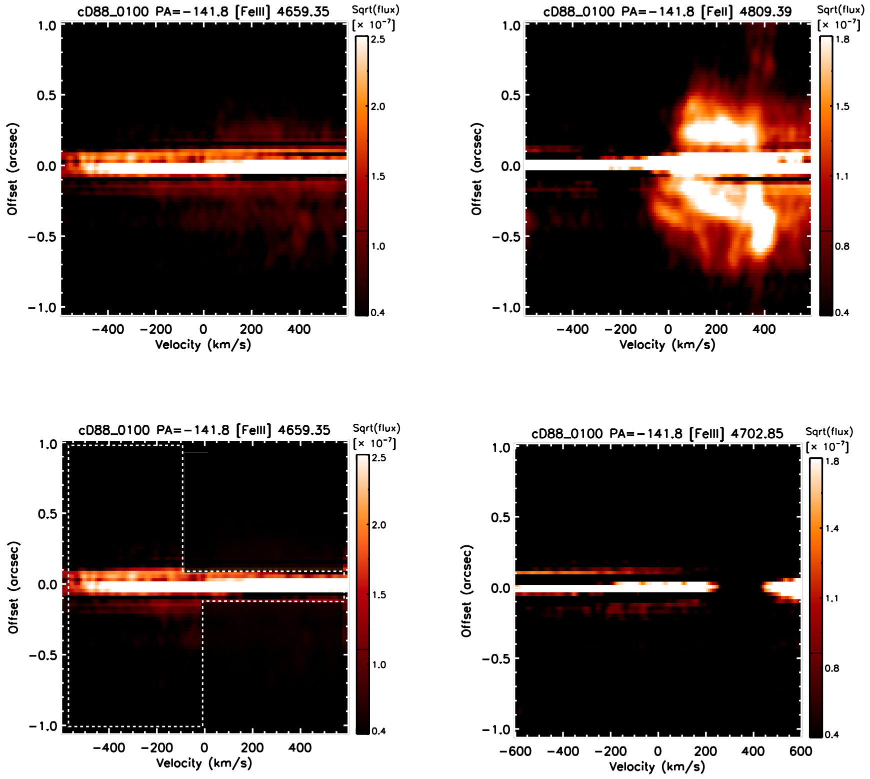


**Figure A17.** Same as Figures A14 through A16, but for spectro-images recorded 2003 November 17 ($\phi = 1.068$) at STIS slit PA $= -142°$.

## APPENDIX B: FORBIDDEN-LINE EMISSION THEORY

In order to provide context for the discussions of the observations and 3-D modeling, we review here the basic theory for the formation of forbidden lines. The following is based on discussions in Osterbrock (1989) and Dopita & Sutherland (2003).

### B1 Collisional Excitation and the Two-Level Atom

In most nebulae, the majority of atoms of a particular element and ionization state are in the ground state. Any excited states are typically the result of collisions with electrons. The collisional excitation timescale is usually long enough to allow excited atoms to decay back to the ground state via radiative processes. At low enough densities, this is true even if the excited state has a radiative lifetime of several seconds, which is frequently the case for 'forbidden' transitions in ionized plasmas (Dopita & Sutherland 2003). Under such conditions, the flux in an emission line depends on the number of collisions, which is proportional to the product of the number densities of the two colliding species and the probability that a collision will produce collisional excitation (Dopita & Sutherland 2003). This probability depends on the collisional excitation cross section integrated over the energy distribution of the colliding species, which is determined by the temperature $T$.

At high enough densities, collision timescales are short and the population of any upper level is set by the balance between collisional excitation and collisional de-excitation out of the level. In this case, the Boltzmann equilibrium equation,

$$\frac{N_j}{N_1} = \frac{g_j}{g_1} \exp\left(\frac{-\chi}{kT}\right) \,, \tag{B1}$$

determines the populations in the excited states, where $N_j/N_1$ is the ratio of the number densities of atoms in any excited state $j$ compared to those in the ground state $j = 1$, $k$ is the Boltzmann constant, $g_j$ is the statistical weight of the state, and $\chi$ is the energy difference between the ground and excited states (Dopita & Sutherland 2003). For intermediate densities where the collisional and radiative decay rates are comparable, the intensity of an emission line is determined by both the temperature and density.

Consider an idealized atom consisting of only two energy states (a 'two-level' atom), denoting the lower level by '1' and the excited upper level by '2'. Electrons can collisionally excite the atom into an upper level, and once there, if left alone, the atom will return to the ground state via a radiative transition. However, if the excited atom experiences another collision with an electron, it may de-excite back down to the ground state. Recombination/photoionization processes are neglected since the rates for such processes are typically much smaller than the collisional excitation rate (Hillier 1988; Ignace & Brimeyer 2006). While such a two-level atom is very simple, in most hot stellar winds and CWBs, highly non-local thermodynamic equilibrium (non-LTE) conditions exist which allow the two-level atom to be an excellent approximation (Hillier 1988; Ignace & Brimeyer 2006; Ignace et al. 2009).

For a two-level atom, the collisional cross section for excitation, $\sigma_{12}(v)$, is a function of electron velocity $v$ and is zero below the threshold energy $\chi = h\nu_{21}$, where $\nu_{21}$ is the frequency of the line transition. It is typically more convenient to express $\sigma_{12}(v)$ in terms of the collision strength $\Omega_{12}$:

$$\sigma_{12}(v) = \frac{\pi\hbar^2}{m_e^2 v^2}\frac{\Omega_{12}}{g_1} \;\; \text{for} \;\; \frac{1}{2}mv^2 > \chi \,, \tag{B2}$$

where $m_e$ is the electron mass and $\Omega_{12}$ is a function of $v$, but is often approximately constant near $\chi$ (Osterbrock 1989). An important advantage of using $\Omega_{12}$ is that because of symmetry between the upper and lower states, $\Omega_{12} = \Omega_{21}$ (Dopita & Sutherland 2003). The collision strengths must be computed quantum mechanically, but numerous values for most relevant transitions are in the literature (Osterbrock 1989).

### B2 The Critical Density

The general form of the equilibrium equation for the balance between the excitation and de-excitation rates of an excited level is

$$n_e N_1 q_{12} = n_e N_2 q_{21} + N_2 A_{21} \,, \tag{B3}$$

where $n_e$ is the electron number density and $A_{21}$ is the radiative transition probability downwards. The variables $q_{12}$ and $q_{21}$ are the collisional excitation and de-excitation coefficients, respectively, and have units of cm$^3$ s$^{-1}$. In general,

$$q_{12} = q_{21}\frac{g_2}{g_1}\exp\left(\frac{-\chi}{kT}\right) \,, \; q_{12} \neq q_{21} \,. \tag{B4}$$

Solving Equation (B3) for the population ratio one finds

$$\frac{N_2}{N_1} = \frac{n_e q_{12}}{n_e q_{21} + A_{21}} \,. \tag{B5}$$

Note that there exists a critical electron density, $n_c$, at which the radiative depopulation rate matches the collisional de-excitation rate, i.e. from Equation (B3), $n_c N_2 q_{21} = N_2 A_{21}$. This yields the definition of the critical density

$$n_c \equiv \frac{A_{21}}{q_{21}} \,. \tag{B6}$$

Alternatively, the critical condition may be written as $A_{21} = R_{21}$, where $R_{21}$ (cm$^{-3}$ s$^{-1}$) is the collisional de-excitation rate per unit volume. Then,

$$N_2 A_{21} = \beta\frac{\Omega_{12}}{g_2}T^{-1/2} n_c N_2 \,, \tag{B7}$$

where $\beta \equiv [(2\pi\hbar^4)/(k m_e^3)]^{1/2}$, and the critical density becomes

$$n_c = \frac{A_{21} g_2 T^{1/2}}{\beta\Omega_{12}} \,, \tag{B8}$$

the same as Equation (B6) (Dopita & Sutherland 2003). For cases when $n_e < n_c$, collisional de-excitation of the excited level is negligible, while for $n_e > n_c$ it is important. For $n_e = n_c$, collisional de-excitation happens as often as radiation, and so by definition, half of the emission comes from material at the critical density.

### B3 Limiting Behavior of the Forbidden Line Emissivity

It is instructive to briefly examine the behavior of Equation (11) in the two limits $n_e \gg n_c$ and $n_e \ll n_c$. In the high density limit of $n_e \gg n_c$, the last exponential term in the brackets goes to zero and

$$j \approx \frac{\chi A_{21} Q_{i,E} A_E \gamma_e}{4\pi} \, n_e \left(\frac{g_2}{g_1}\right) \exp\left(\frac{-\chi}{kT}\right) \; . \qquad \text{(B9)}$$

Thus, the emissivity scales with the density $n_e$, approaching a constant for high values of $T$. However, at low $T$, the exponential term dominates and the line fades rapidly with decreasing $T$.

In the opposite limit of $n_e \ll n_c$, doing a series expansion of the last term in brackets in Equation (11) yields

$$\begin{aligned} j &\approx \frac{\chi A_{21} Q_{i,E} A_E \gamma_e}{4\pi} \, n_e \left(\frac{g_2}{g_1}\right) \left(\frac{n_e}{n_c}\right) \exp\left(\frac{-\chi}{kT}\right) \\ &= \frac{\chi Q_{i,E} A_E \gamma_e \beta}{4\pi} \, n_e^2 \left(\frac{\Omega_{12}}{g_1}\right) T^{-1/2} \exp\left(\frac{-\chi}{kT}\right) \; . \qquad \text{(B10)} \end{aligned}$$

In this case, the emissivity scales with $n_e^2$, reaching a maximum at a temperature $T = 2\chi/k$. At low $T$, the exponential term dominates, and the line rapidly fades with decreasing $T$. For high $T$, the $T^{-1/2}$ term dominates and the line slowly fades with increasing $T$.

This paper has been typeset from a TEX/ LATEX file prepared by the author.
